# Supplementary material for: Data-Free Quantization Through Weight Equalization and Bias Correction
Source: arXiv:1906.04721 source file (2019-11-25)
Supplement: Supplementary file 1 [file appendix-equalization.tex]

Consider two fully-connected layers with weight matrices $\mat{W^{(1)}}$ and $\mat{W^{(2)}}$, that we scale as in \ref{sec:positivescalingequivariance}. We investigate the problem of optimizing the quantization ranges by rescaling the weight matrices by $\mat{S} = diag(\vec{s})$, where $\vec{s} > 0$, such that $\mat{\bar{W}^{(1)}} = \mat{W^{(1)}} \mat{S}$ and $\mat{\bar{W}^{(2)}} = \mat{S^{-1}}\mat{W^{(2)}} $ the weight matrices after rescaling. We investigate the case of symmetric quantization, which also gives good results in practice for asymmetric quantization. We denote
\begin{align}
\vec{r^{(1)}} &= max_i |\mat{W}^{(1)}_{(i, j)}\mat{S}| \\
\vec{r^{(2)}} &= max_j |\mat{S^{-1}}\mat{W}^{(2)}_{(i, j)}| \\
R^{(k)} &= max_i (\vec{r}_i^{(k)})
\end{align}
Where $\vec{r^{(k)}}$ is the per-channel weight quantization range that is scaled by $\mat{S}$, and $\vec{R^{(k)}}$ the activation range for the full weight matrix $\mat{W^{(k)}}$. We also define $\hat{\vec{r}}^{(k)}$ the original unscaled ranges.\\
We investigate the relative errors between the tensor activation range, and channel activation range
\begin{align}
    e^{(k)}_i = \frac{R^{(k)}_i - r^{(k)}_i}{R^{(k)}_i} = 1 - \frac{ r^{(k)}_i}{R^{(k)}_i}
\end{align}
And want to optimize all the ranges such that
\begin{align}
    \mathcal{E} = \max_{\mat{S}}\sum_i e^{(1)}_i \cdot e^{(2)}_i \label{eq:opt}
\end{align}
This spreads out the relative error as much as possible over matrix $1$ and $2$.

We note that for an optimal solution $\mat{S}$, scaling $\alpha \mat{S}$ also gives an optimal solution, as $\alpha$ cancels out in $\mathcal{E}$. So we can choose a solution such that $R = R^{(1)} = R^{(2)}$. \iffalse Combining this with the above statement, we have that for any solution after $\alpha$ scaling, we can find some $i$ such that $r_i^{(1)} = r_i^{(2)} = R^{(1)} = R^{(2)}$, such that $\forall k \neq i: r_i^{(1)} \cdot r_i^{(2)}> r_k^{(1)} \cdot r_k^{(2)}$. This defines for us the maximum $R$ after our rescaling procedure.\\ \fi
Now, given this $R$, we see that optimizing eq. \ref{eq:opt} is now independent for each $i$th term in $\mathcal{E}$. For each term we calculate
\begin{align}
    &\max_{s_i} e_i^{(1)} \cdot e_i^{(2)} = \\
    &\max_{s_i} (1 - \frac{r_i^{(1)}}{R})(1 - \frac{r_i^{(2)}}{R}) =  \\
    &\max_{s_i} -s_i \hat{r}_i^{(1)} - s_i^{-1}\hat{r}_i^{(2)} 
\end{align}
Differentiating with respect to $s_i$ and setting equal to zero gives $s_i = \frac{1}{\hat{r}_i^{(1)}}\sqrt{\hat{r}_i^{(1)} \hat{r}_i^{(2)}}$.
