# Supplementary material for: Data-Free Quantization Through Weight Equalization and Bias Correction
Source: arXiv:1906.04721 source file (2019-11-25)
Supplement: Supplementary file 2 [file appendix.tex]

\subsection{Derivation for piece-wise linear functions}

More generally, this scaling invariance hold for the all piece-wise linear activations functions if the splitting points and offsets are scaled according to $s$.

\begin{equation}
    f(x)=
    \begin{cases}
        a_1 x + b_1 &\text{if } x \leq c_1\\
        a_2 x + b_2 &\text{if } c_1 < x \leq c_2\\
        &\vdots \\
        a_n x + b_n &\text{if } c_{n-1} < x
    \end{cases}
\end{equation}

\begin{align}
    f(sx) &=
    \begin{cases}
        a_1 sx + b_1 &\text{if } sx \leq c_1\\
        a_2 sx + b_2 &\text{if } c_1 < sx \leq c_2\\
        &\vdots \\
        a_n sx + b_n &\text{if } c_{n-1} < sx
    \end{cases}\\
    &= s
    \begin{cases}
        a_1 x + b_1 / s &\text{if } x \leq c_1 / s\\
        a_2 x + b_2 / s &\text{if } c_1 / s < x \leq c_2 / s\\
        &\vdots \\
        a_n x + b_n / s &\text{if } c_{n-1} / s < x
    \end{cases}
\end{align}
From this follows that $f(sx) = s \Tilde{f}(x)$ where $\Tilde{b}_i = b_i/s$ and $\Tilde{c}_i = c_i/s$.

\subsection{Show scaling}
\todo{do we need it?}
We make use of a linear-scaling invariant property between subsequent layers in a neural network. Given input $X$ and two linear layers with weights $W_1$, $W_2$ \iffalse and biases $b_1$, $b_2$ \fi, we can always move around scaling factors $s$ from the columns of $W_1$ to the rows of $W_2$ while keeping the overall computation exactly the same.

\small
\begin{align*}
&r \left(
\left[
  \begin{array}{ccc}
    \horzbar & w_{1} & \horzbar \\
    \horzbar & w_{2} & \horzbar \\
    \horzbar & \vdots & \horzbar \\
    \horzbar & w_{n} & \horzbar \\  
  \end{array}
\right]_2
r \left(
\left[
  \begin{array}{cccc}
    \vrule & \vrule & & \vrule\\
    w_{1} & w_{2} & \ldots & w_{n} \\
    \vrule & \vrule & & \vrule 
  \end{array}
\right]_1
\begin{bmatrix}
           x_{1} \\
           x_{2} \\
           \vdots \\
           x_{m}
         \end{bmatrix}
         \right)
         \right)
         =           \\
&r \left(
\left[
  \begin{array}{ccc}
    \horzbar & w_{1} & \horzbar \\
    \horzbar & w_{2} \cdot s & \horzbar \\
    \horzbar & \vdots & \horzbar \\
    \horzbar & w_{n} & \horzbar \\  
  \end{array}
\right]_2
r \left(
\left[
  \begin{array}{cccc}
    \vrule & \vrule & & \vrule\\
    w_{1} & w_{2} \cdot \frac{1}{s} & \ldots & w_{n} \\
    \vrule & \vrule & & \vrule 
  \end{array}
\right]_1
\begin{bmatrix}
           x_{1} \\
           x_{2} \\
           \vdots \\
           x_{m}
         \end{bmatrix}
         \right)
         \right)
         \\
\end{align*}
\normalsize

where r is the ReLU function. This can also be done with any other piecewise linear activation function. %Prove/indicate this.
% Add how biases get into this picture as well\\
By rescaling this way many times across layers, we can take the maximum element of one weight matrix, scale it by $1/s$ and absorb $s$ in any of it's adjacent layers. Effectively reducing the magnitude of the maximum weigh in the original matrix, while keeping the computation exactly the same.
